# Supplementary material for: Nodal pair density waves from a quarter-metal in crystalline graphene multilayers
Source: arXiv:2210.15660 ancillary file (2025-08-14)
Supplement: Supplementary file 1 [file Supplementary.pdf]

# Supplementary Materials: Nodal pair-density-waves from quarter metal in crystalline graphene multilayers

Sk Asrap Murshed,<sup>1,\*</sup> András L. Szabó,<sup>2,\*</sup> and Bitan Roy<sup>1</sup>

<sup>1</sup>*Department of Physics, Lehigh University, Bethlehem, Pennsylvania, 18015, USA*

<sup>2</sup>*Institute for Theoretical Physics, ETH Zürich, 8093 Zürich, Switzerland*

(Dated: October 27, 2022)

In this Supplementary Materials, we derive the low energy Hamiltonian for BBLG and RTLГ by including the valley and spin degrees of freedom, and accounting for the momentum-independent effect of the electric displacement field. Subsequently, we add the requisite orderings to lift the four-fold spin and valley degeneracy of electronic bands, which in turn allows us to compute the momentum-independent band gap in the quarter-metal phase in these two systems.

## S1. AMPLITUDE OF THE UNIFORM MASS IN QUARTER-METAL (QM) OF BBLG AND RTLГ

In this Supplementary Materials we elaborate on the origin of the momentum-independent part of the mass term  $m(0) \equiv m_0$  in Eq. (7) of the main text. The lifting of four-fold spin and valley degeneracy leading to the formation of the QM in BBLG and RTLГ is due to the presence of three competing orders, represented by mutually commuting matrix operators. To see this, we first restore the valley and spin degrees of freedom. Subsequently, we use this enlarged Hilbert space to introduce the pertinent order parameters.

To describe spinful electrons near two inequivalent valleys at  $\pm\mathbf{K}$  we enlarge the original two-component spinor to an eight component one as

$$\Psi = [c_a, c_b]^\top \rightarrow [c_{a\uparrow}^{+\mathbf{K}}, c_{b\uparrow}^{+\mathbf{K}}, c_{a\uparrow}^{-\mathbf{K}}, c_{b\uparrow}^{-\mathbf{K}}, c_{a\downarrow}^{+\mathbf{K}}, c_{b\downarrow}^{+\mathbf{K}}, c_{a\downarrow}^{-\mathbf{K}}, c_{b\downarrow}^{-\mathbf{K}}]^\top, \quad (\text{S1})$$

where  $c_{\beta,\sigma}^{\tau\mathbf{K}}$  annihilates an electron on sublattice  $\beta = a, b$  with spin projection  $\sigma = \uparrow, \downarrow$  and at valley  $\tau\mathbf{K}$ , where  $\tau = \pm$ . We write the eight-dimensional Hermitian matrices operating on this Hilbert space as a Kronecker product  $\Gamma_{\mu\nu\lambda} = \sigma_\mu \otimes \tau_\nu \otimes \beta_\lambda$  with Pauli matrices  $\{\sigma_\mu\}$ ,  $\{\tau_\nu\}$  and  $\{\beta_\lambda\}$  acting on spin, valley, and sublattice degrees of freedom, respectively. Here  $\mu, \nu, \lambda = 0, 1, \dots, 3$  and 0 index corresponds to the a two-dimensiona unit matrix.

The Taylor expansion analogous to Eq. (7) but about the opposite  $-\mathbf{K}$  valley can be obtained using valley reflection symmetry under which  $(k_x, k_y) \rightarrow (-k_x, k_y)$ . Consequently the  $p$ -,  $d$ -, and  $f$ -wave harmonics change according to

$$p_1 \rightarrow -p_1, \quad p_2 \rightarrow p_2, \quad d_1 \rightarrow d_1, \quad d_2 \rightarrow -d_2, \quad f_1 \rightarrow -f_1, \quad f_2 \rightarrow f_2. \quad (\text{S2})$$

Furthermore, as we neglect the spin-orbit coupling in BBLG and RTLГ, spin degrees of freedom merely doubles in the Hamiltonian. Then, the normal state Hamiltonian featuring fourfold (valley and spin) degenerate bands reads

$$H = \alpha_0 \Gamma_{001} + \alpha_1 (\Gamma_{031} p_1 + \Gamma_{002} p_2) + \alpha_2 (\Gamma_{001} d_1 - \Gamma_{032} d_2) + \alpha_3 (\Gamma_{031} f_1 - \Gamma_{002} f_2) + \alpha_{12} d_2 (\Gamma_{031} p_2 + \Gamma_{002} p_1) + V \Gamma_{003}, \quad (\text{S3})$$

which is gapped by the electric field term proportional to  $V$ .

Now we consider the effect of the dominant channels of electronic interactions. Repulsive on-site Hubbard  $U$  in graphene heterostructures induces a layer (or sublattice) antiferromagnet ordering with amplitude  $\Delta_{\text{LAF}}$ , described by the matrix operator  $\Delta_{\text{LAF}} \Gamma_{303}$ , where we arbitrarily (without any loss of generality) choose the spin quantization along the  $z$  axis. Both the  $V$  and  $\Delta_{\text{LAF}}$  terms introduce a spectral gap. However, due to the commutation of the corresponding matrix operators  $[\Gamma_{003}, \Gamma_{303}] = 0$ , the simultaneous presence of these orderings lifts the spin-degeneracy, but maintains the valley degeneracy. And for low doping we realize a spin-polarized half-metal [1, 2].

---

\* Equal contributors

The next relevant component of short-range interactions is intralayer second-nearest neighbor Hubbard repulsion, which in the spin-polarized system induces quantum anomalous Hall ordering with amplitude  $\Delta_{\text{QAH}}$ , described by the operator  $\Delta_{\text{QAH}}\Gamma_{033}$  [3]. As  $[\Gamma_{033}, \Gamma_{003}] = [\Gamma_{033}, \Gamma_{303}] = 0$ , this Haldane mass represents yet another commuting order. Therefore, a simultaneous presence of these three orderings lifts the complete fourfold degeneracy of the normal state band structure [1, 2]. The Hamiltonian operator in the presence of these three orders reads as

$$H = \alpha_0\Gamma_{001} + \alpha_1(\Gamma_{031}p_1 + \Gamma_{002}p_2) + \alpha_2(\Gamma_{001}d_1 - \Gamma_{032}d_2) + \alpha_3(\Gamma_{031}f_1 - \Gamma_{002}f_2) + \alpha_{12}d_2(\Gamma_{031}p_2 + \Gamma_{002}p_1) + V\Gamma_{003} + \Delta_{\text{LAF}}\Gamma_{303} + \Delta_{\text{QAH}}\Gamma_{033}. \quad (\text{S4})$$

Assuming  $V > \Delta_{\text{LAF}} > \Delta_{\text{QAH}}$ , the gap between the bands closest to zero energy has the magnitude  $2|V - \Delta_{\text{LAF}} - \Delta_{\text{QAH}}|$ , which constitutes the momentum-independent part of the mass  $m_0 = |V - \Delta_{\text{LAF}} - \Delta_{\text{QAH}}|$  in the QM phase. As mentioned in the main text, interlayer nearest neighbor Hubbard repulsion in graphenelike systems introduces charge-density-wave or sublattice polarization of electronic density between two layers. However, this symmetry is already broken by the electric field.

- 
- [1] A. L. Szabó and B. Roy, Phys. Rev. B **105**, L081407 (2022).
  - [2] A. L. Szabó and B. Roy, Phys. Rev. B **105**, L201107 (2022).
  - [3] A. L. Szabó and B. Roy, Phys. Rev. B. **103**, 205135 (2021).
